# Supplementary material for: The History and Risks of Reinforcement Learning and Human Feedback
Source: arXiv:2310.13595 source file (2023-11-28)
Supplement: Supplementary file 1 [file 99_appendix.tex]

\newpage
\appendix
\section{Appendices}

\subsection{Additional Resources}
Richard Sutton has created a useful history of reinforcement learning here that provides more detail than our work: \url{http://incompleteideas.net/book/ebook/node12.html}

TODO collect more references
\subsection{Human-in-the-loop RL and RLHF}
``A social reinforcement learning agent''~\citep{isbell2001social}

\subsection{Further 
 history}
